# Supplementary material for: Reanalyses and a high-resolution model fail to capture the `high tail' of CAPE distributions
Source: arXiv:2012.13383 ancillary file (2020-12-24)
Supplement: Supplementary file 1 [file Wang_Moyer_2020_CAPE_Distribution_suppdocs.pdf]

# Reanalyses and a high-resolution model fail to capture the 'high tail' of CAPE distributions
# Supplemental material

Ziwei Wang, James A. Franke, Zhenqi Luo, Elisabeth J. Moyer

December 8, 2020

## 1 CAPE distributions and biases

| | | IGRA | ERAI | ERA5 | WRF |
|---|---|---|---|---|---|
| SBCAPE | w/ zeroes | 303.1 | 309.9 | 320.1 | 308.7 |
| | w/o zeroes | 755.4 | 798.6 | 781.2 | 791.7 |
| MUCAPE | w/ zeroes | 487.8 | 371.4 | 383.2 | 349.5 |
| | w/o zeroes | 990.0 | 909.1 | 900.0 | 877.5 |
| MLCAPE | w/ zeroes | 249.3 | 201.6 | 208.1 | 202.7 |
| | w/o zeroes | 694.1 | 626.8 | 628.0 | 629.8 |
| Corrected SBCAPE | w/ zeroes | 303.1 | 286.7 | 305.3 | 293.3 |
| | w/o zeroes | 755.4 | 799.4 | 763.2 | 797.6 |

Table S1: Mean values of each type of CAPE (unit: J/kg) from the four datasets considered in this study. All year is shown and are not paired to IGRA. We show averages both with and without zeroes included. Bottom rows is corrected SBCAPE, recomputed with surface values replaced with those measured by radiosondes (a fair amount of data is still not corrected when no observation is available). Note that mean values of model and reanalysis CAPE are slightly larger than in radiosondes, even though these data products substantially underpredict the high tail of CAPE distributions. Overly narrow CAPE distributions may still show reasonable mean values.

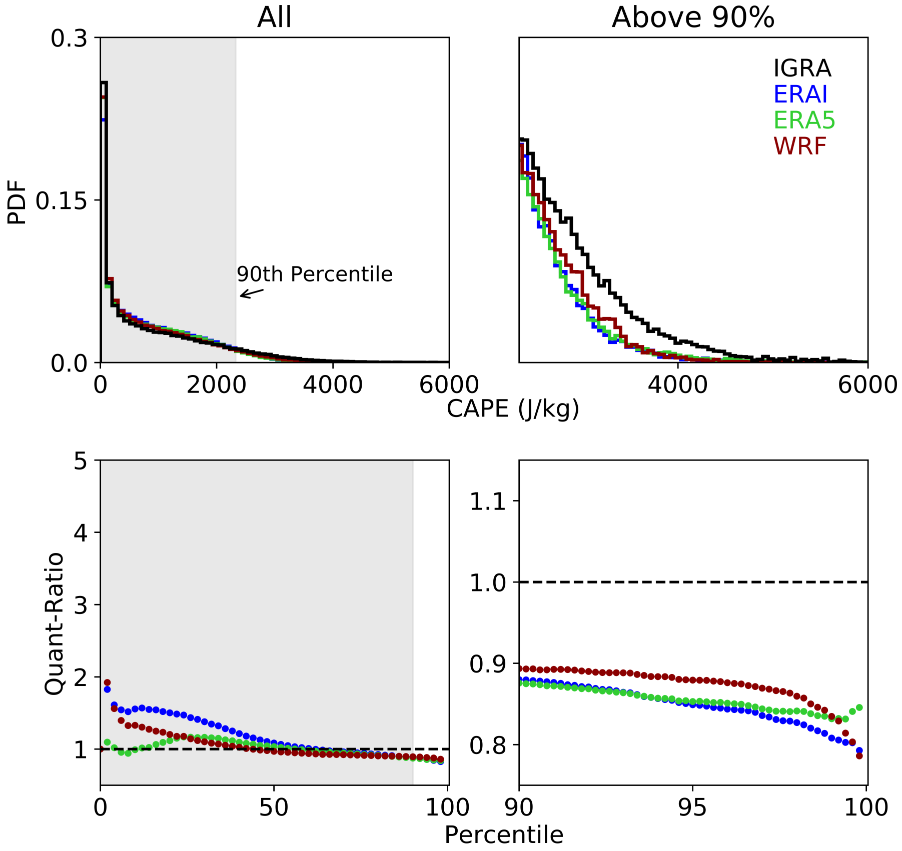


Figure S1: As in manuscript Figure 2, but for MLCAPE instead of SBCAPE. Points with zero CAPE are excluded from the analysis (64–68% of the datasets). PDFs are cut off at 6000 J/kg on x-axis, as less than 0.02% of all points lie above the limit. For IGRA, the 90th percentile is 1914 J/kg, the 95th is 2484 J/kg , and the 97.5th is about 2955 J/kg. Biases in the distribution and mean of MLCAPE are midway between those in SBCAPE and MUCAPE.

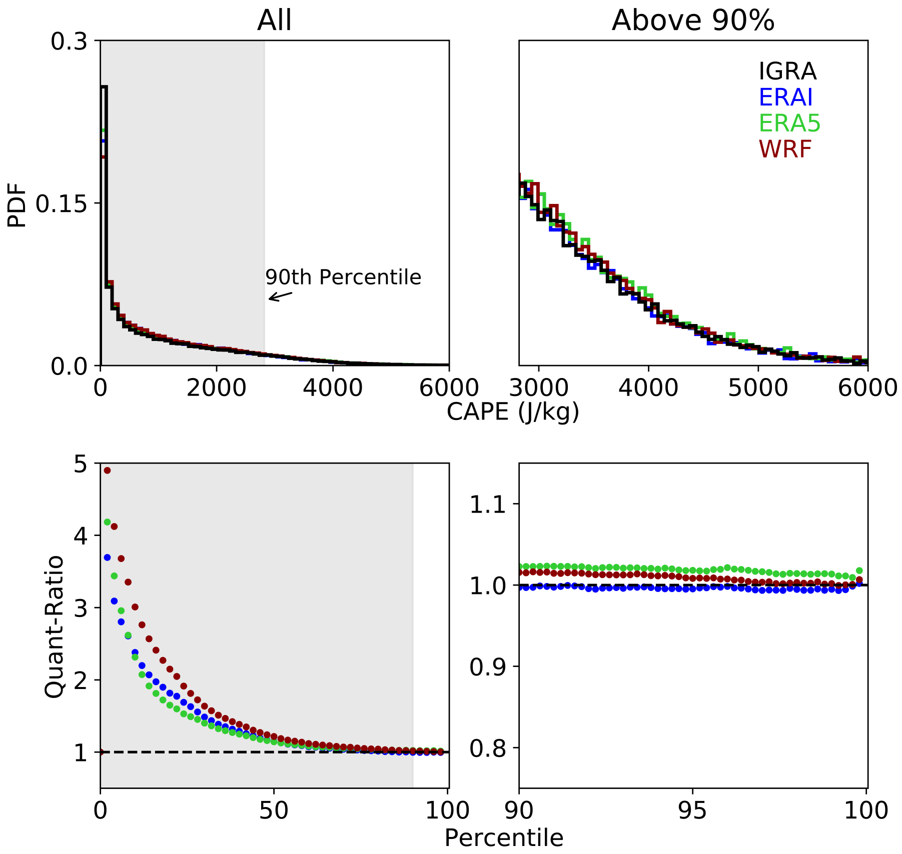


Figure S2: As in manuscript Figure 2, but for corrected instead of uncorrected SBCAPE. Correcting surface temperature and humidity removes discrepancies in the high tail, though model and reanalysis still overpredict CAPE values in the low quantiles.

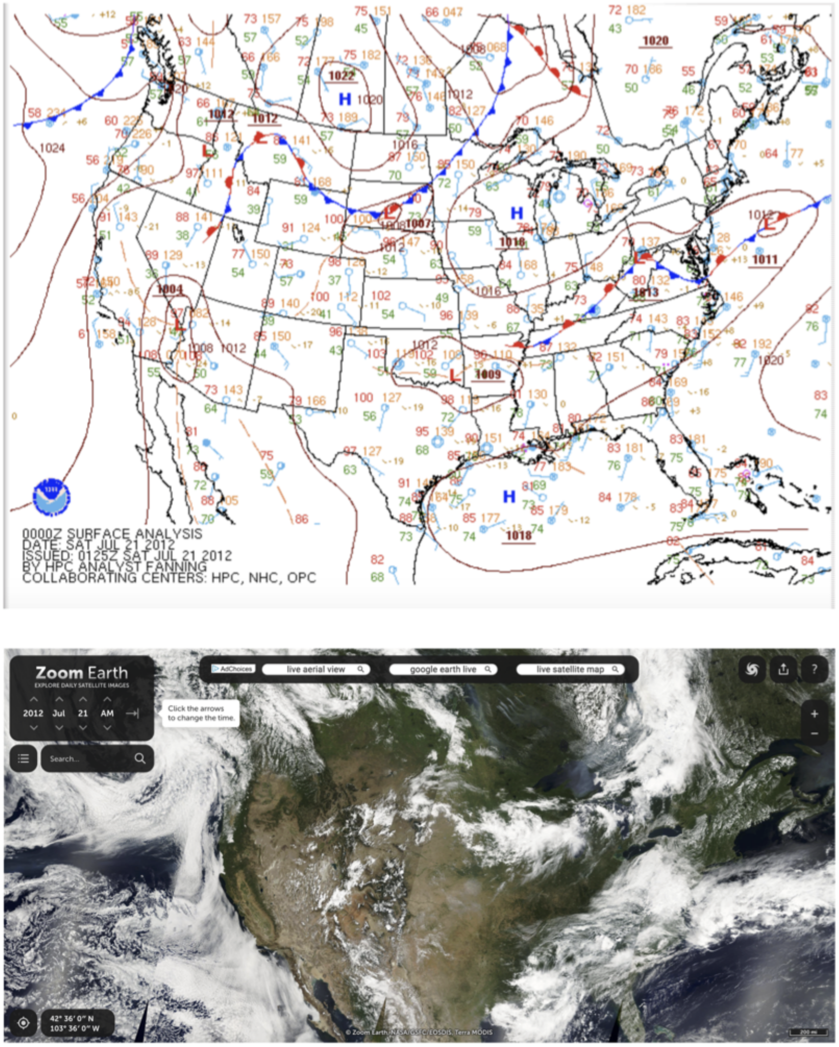


Figure S3: The example day of July 21, 2012 shown as (**top**) a weather map from the National Weather Service (NWS), and (**bottom**) a satellite image from Terra MODIS visualized by Zoom Earth. Compare to manuscript Figure 4. Images are available online at $https://www.wpc.ncep.noaa.gov/archives/web\_pages/sfc/sfc\_archive\_maps.php?arcdate = 07/21/2012\&selmap = 2012072100\&maptype = namussfc$, $https://zoom.earth/\#view = 42.6, -103.6, 4.54z/date = 2012 - 07 - 21, am$. In this time period a stationary front in the Southeast U.S. brings high moisture and cloud cover to the region. Extreme SBCAPE occurs at the edge of this zone, where moist air meets the high temperatures of the Central U.S.

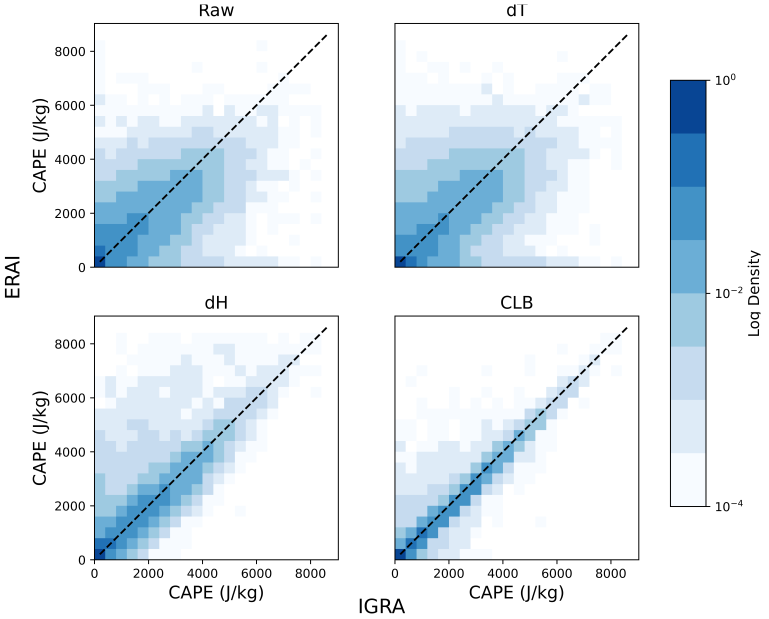


Figure S4: As in manuscript Figure 5, but for ERAI instead of WRF.

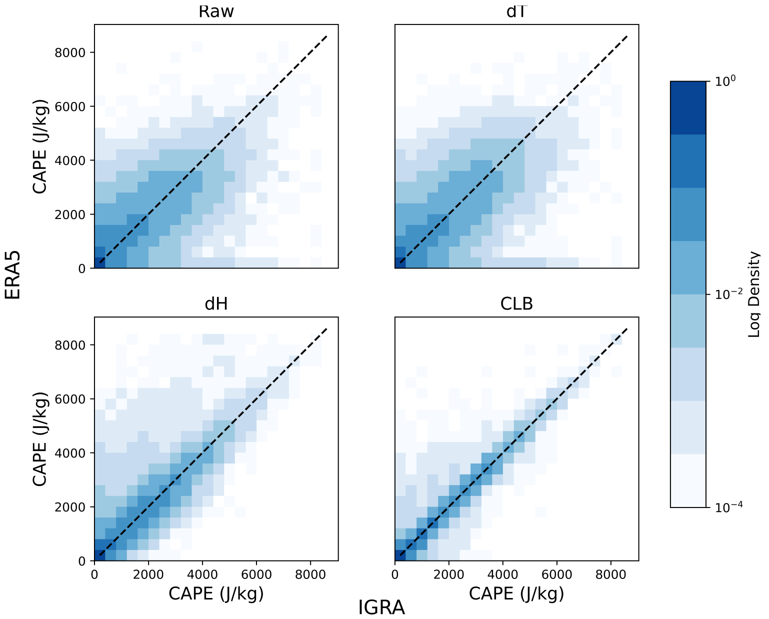


Figure S5: As in manuscript Figure 5, but for ERA5 instead of WRF.

| | ERAI | ERA5 | WRF |
|---|---|---|---|
| Raw | 0.836 | 0.856 | 0.737 |
| dT | 0.840 | 0.866 | 0.712 |
| dH | 0.936 | 0.946 | 0.924 |
| All | 0.989 | 0.989 | 0.988 |

Table S2: Improvement of the SBCAPE match to observations by correcting surface values: table shows Pearson-r for the correlation of CAPE from different datasets against radiosondes, using different surface level corrections. Top to bottom rows show values for raw data, surface temperature and pressure corrected, surface humidity and pressure corrected, and with all surface values corrected. All correlation coefficients pass the two-sided test at 0.1% significance level.

## 2 CAPE as a function of surface T, H

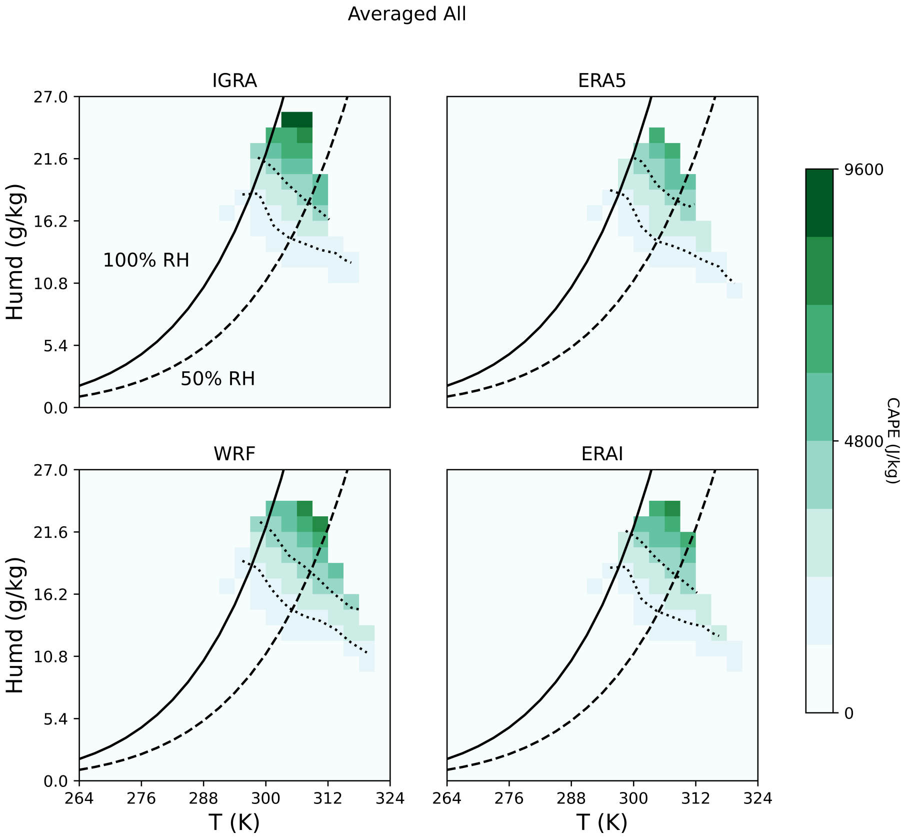


Figure S6: As in manuscript Figure 6, but for all datasets. (Top left) IGRA, (top right) ERA5, (bottom left) WRF, and (bottom right) ERAI. Contours correspond to 2000 and 4000 J/kg. All datasets show similar dependence of SBCAPE on surface temperature and humidity, but IGRA radiosondes sample more extreme (hot, humid) conditions.

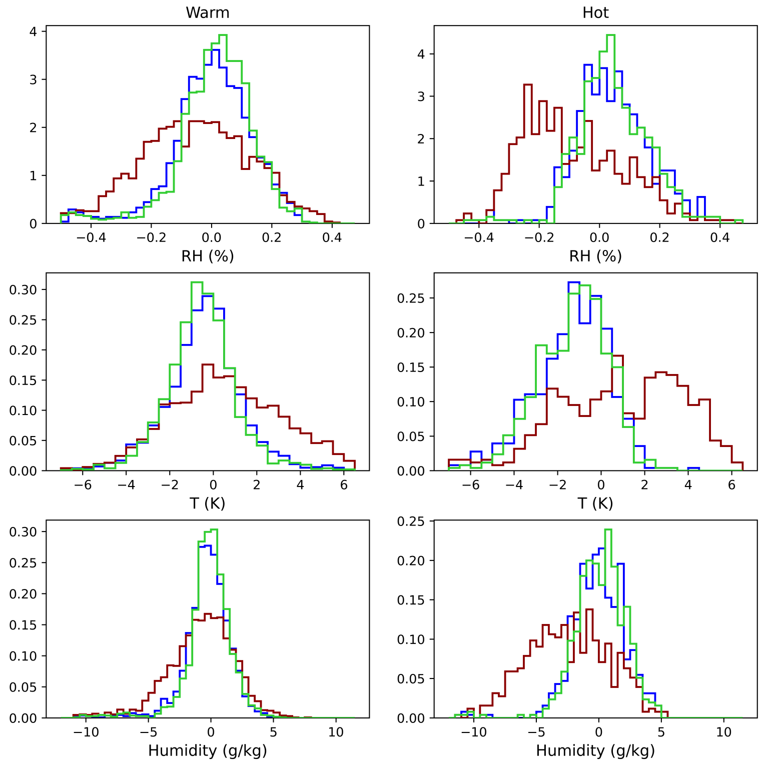


Figure S7: Distributions of errors in reanalysis and model surface values for the ‘warm’ and ’hot’ bins defined in manuscript Figure 7, Figure shows reanalysis and model errors in profiles assigned to these T,H bins based on their radiosonde values. Mean biases are relatively small, especially in reanalyses. As is the norm, reanalyses are slightly too cold and WRF is too hot and dry. The distributions of errors are in most cases reasonably symmetrical, and mean biases are small relative to standard deviations: for example, ERA5 specific humidity in the ’hot’ bin has mean bias of .007 g/kg but error standard deviation 2.3 g/kg. Mean biases, skew in distributions, and standard deviations are largest in WRF. Complete values of mean and error standard deviations are given in Table S3.

| | | ERAI | ERA5 | WRF |
|---|---|---|---|---|
| 'Hot' bin | RH (%) | 4.6 (11.8) | 4.6 (11.1) | -8.8 (15.9) |
| | T (K) | -1.4 (1.9) | -1.3 (1.8) | 0.9 (2.1) |
| | H (g/kg) | -0.07 (2.3) | 0.007 (2.3) | -2.5 (3.4) |
| 'Warm' bin | RH (%) | 0 (12.8) | 1.1 (12.3) | -5.8 (17.9) |
| | T (K) | -0.2 (2.5) | -0.3 (2.5) | 1.0 (2.4) |
| | H (g/kg) | -0.3 (1.9) | -0.2 (1.8) | -0.8 (2.7) |
| Average | RH (%) | -0.4 (12.4) | -0.4 (11.9) | -2.4 (18.3) |
| | T (K) | -0.1 (2.8) | -0.1 (2.5) | 0.3 (3.4) |
| | H (g/kg) | 0.03 (1.3) | 0.04 (1.2) | -0.15 (1.8) |

Table S3: Mean and standard deviation (in parentheses) of errors in reanalysis and models in RH, temperature, and specific humidity, all computed against paired radiosonde soundings as in Figure S7. Values are given for (**top, middle**) the 'hot' and 'warm' bins from Figure S7 and manuscript Figure 7 and (**bottom**) as averages over entire datasets. Standard deviations of profile errors are relatively constant in all cases, presumably because the weather events that produce strong gradients occur in a wide variety of environments. Biases are stronger in the 'hot' bin, which samples warm, humid conditions associated with extreme CAPE.

| | IGRA | ERAI | ERA5 | WRF |
|---|---|---|---|---|
| RH (%) | 68.4 | 67.9 | 68.0 | 65.9 |
| T (K) | 286.6 | 286.5 | 286.5 | 287.0 |
| H (g/kg) | 7.65 | 7.68 | 7.68 | 7.50 |

Table S4: Mean values of RH, temperature, and specific humidity for paired profiles in four datasets considered in this study. Mean biases are small, though the WRF hot and dry bias is evident. However, biases in surface values show strong distributional effects; see Figures S9-S10.

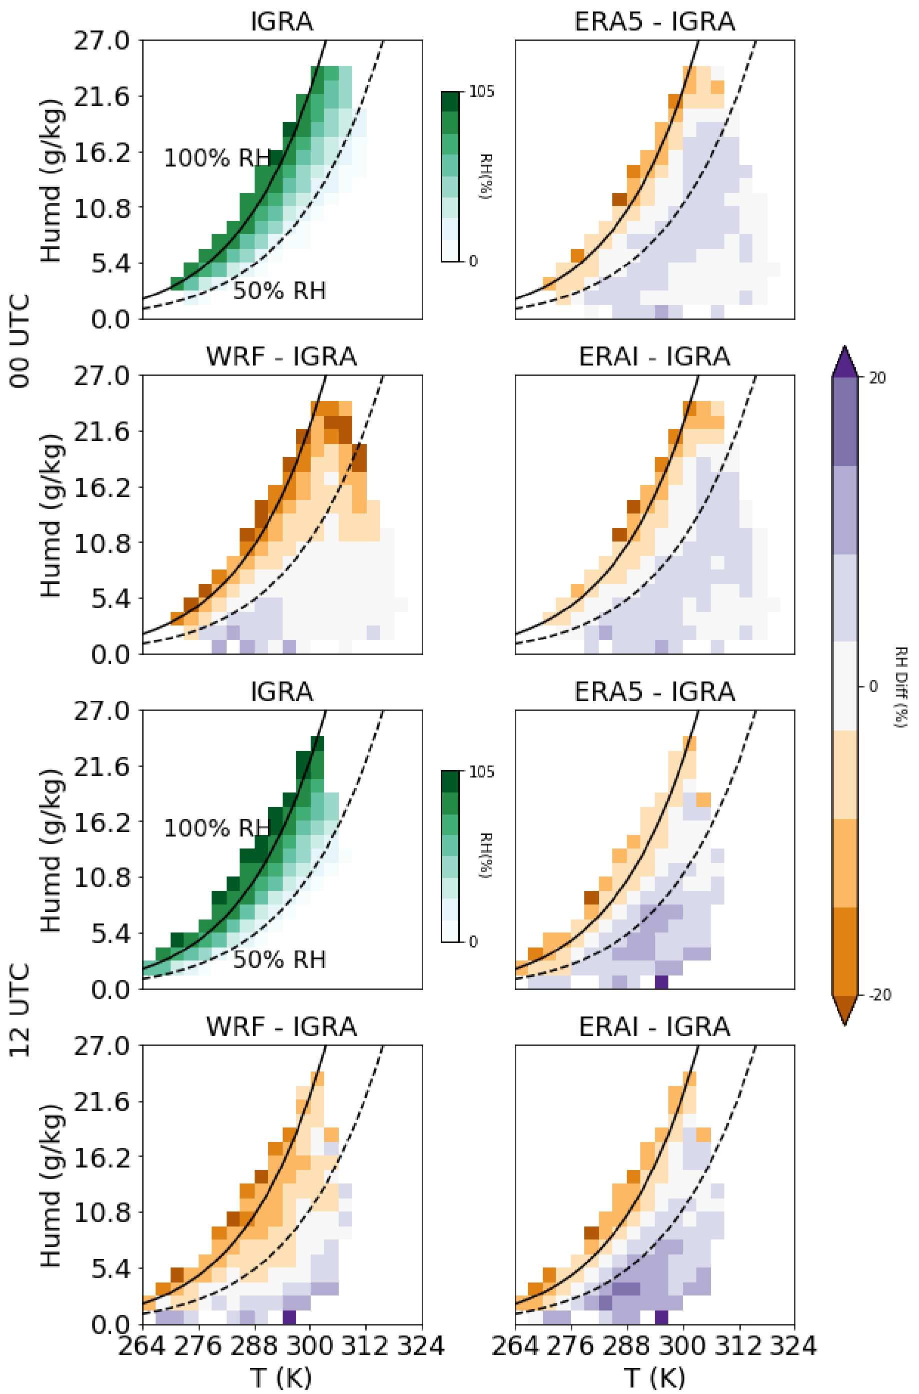


Figure S8: Relative humidity biases in reanalyses and model in T-H space, as in manuscript Figure 8–9 but here we show not under- or over-prediction of T,H incidences but the mean absolute bias of profiles matched to radiosonde soundings. Top and bottom groups of four subplots are soundings at 00 and 12 UTC. Solid and dashed lines mark 100% and 50% RH. In each group: (**Top left**) mean RH of radiosonde profiles in each bin. (**Other panels**) mean RH bias for (clockwise from top right) ERA5, ERAI, and WRF relative to paired radiosonde profiles. Reanalyses and model underestimate RH in moist (high RH) soundings and overestimate it in dry ones. Overall, RH biases are correlated with those in temperature: compare to Figure S9.

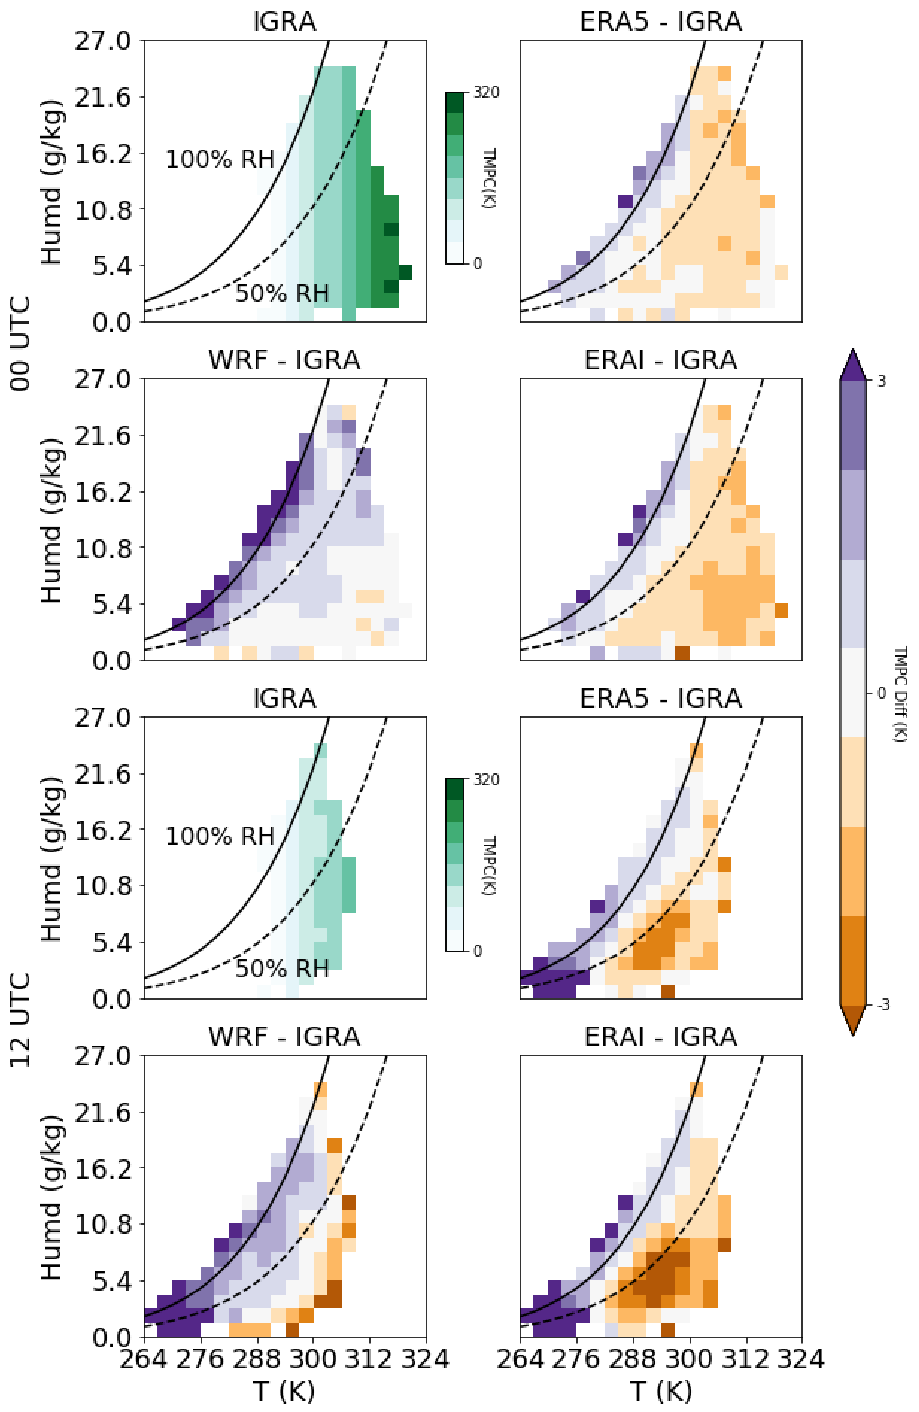


Figure S9: As in Figure S8 but here for temperature biases. Top and bottom groups of four subplots are soundings at 00 and 12 UTC. In each group: (**Top left**) mean temperature of radiosonde profiles in each bin. Since the x axis is T, values are simply ordered horizontally. (**Other panels**) mean temperature bias for (clockwise from top right) ERA5, ERAI, and WRF relative to paired radiosonde profiles. In true moist (high RH) soundings, both ERA and WRF overpredict temperature (purple). In true dry (low RH) soundings, ERA reanalyses underpredict temperature (yellow).

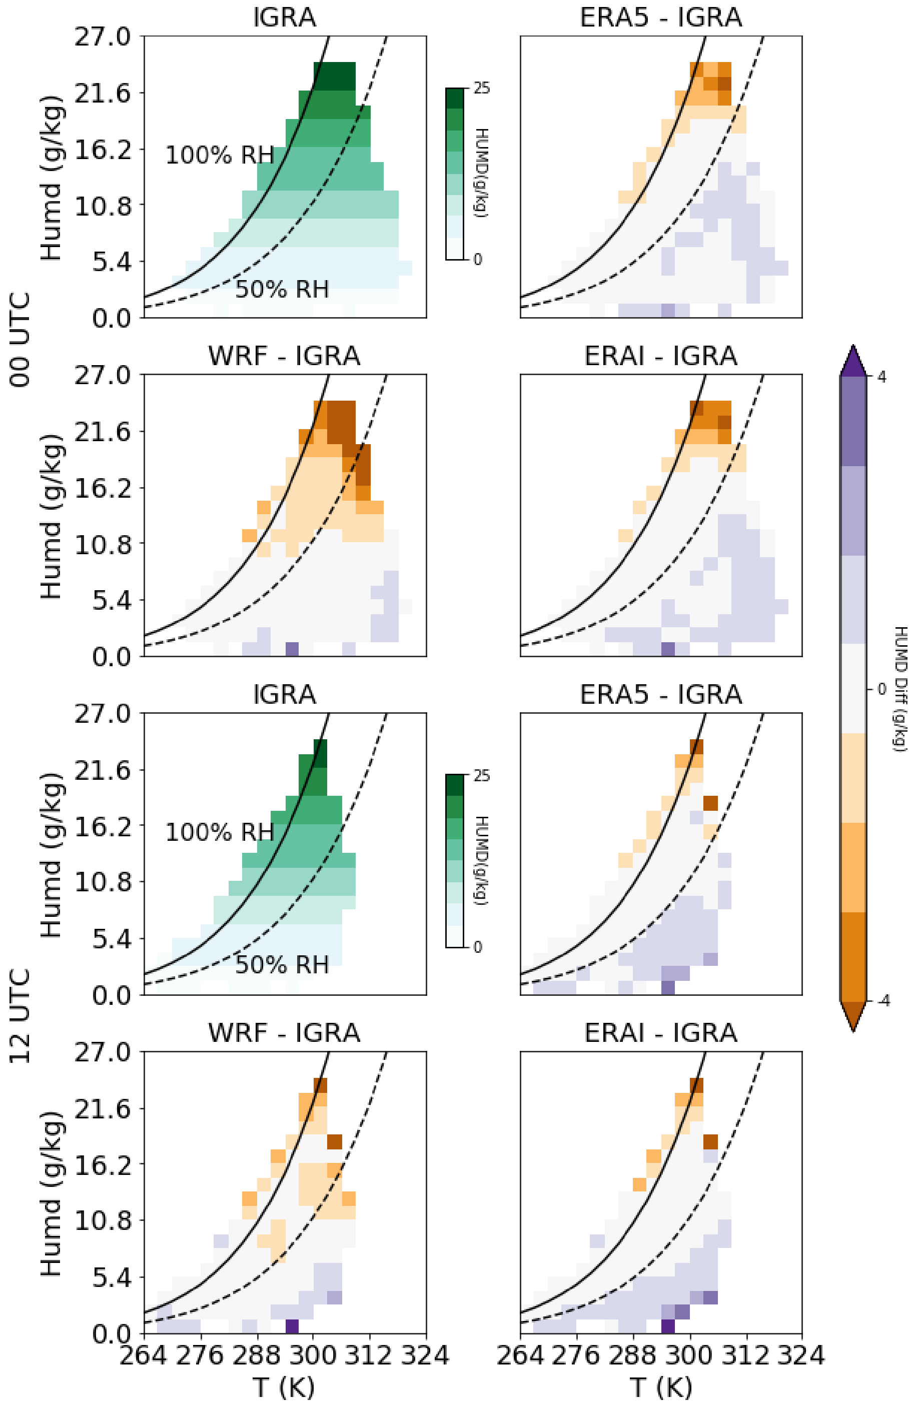


Figure S10: As in Figure S8 but here for specific humidity biases. Top and bottom groups of four subplots are soundings at 00 and 12 UTC. In each group: (**Top left**) mean specific humidity of radiosonde profiles in each bin. Since the y axis is H, values are simply ordered vertically. (**Other panels**) mean H bias for (clockwise from top right) ERA5, ERAI, and WRF relative to paired radiosonde profiles. Reanalyses and model all underestimate humidity in hot, humid soundings, even though temperature biases differ in sign. This bias drives the underprediction of the high tail of CAPE.

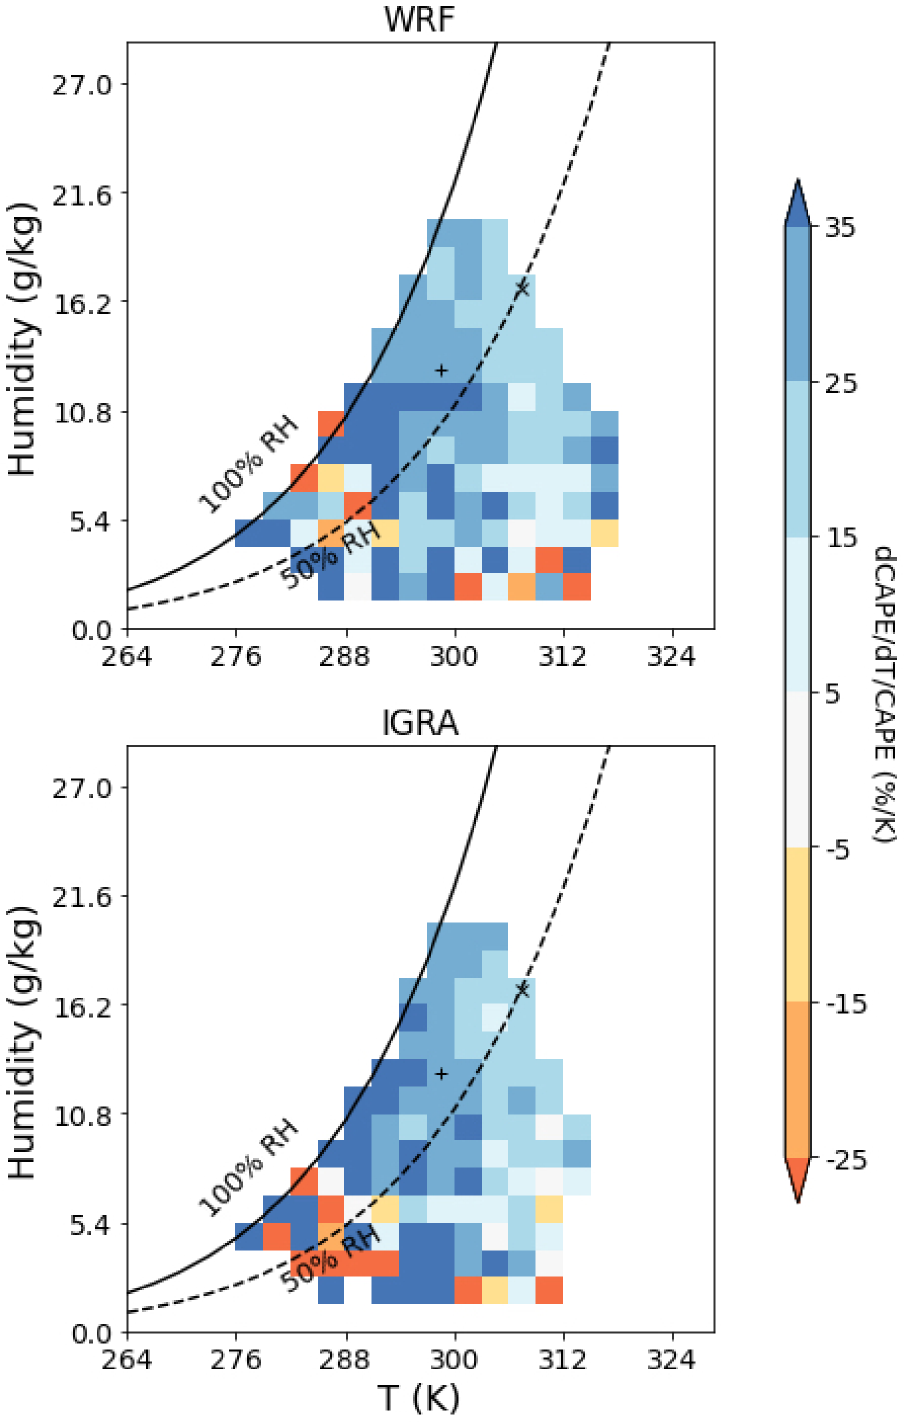


Figure S11: Heatmap of fractional change of CAPE per degree temperature under current climate for (top) WRF and (bottom) IGRA radiosondes. IGRA values are the slope of heatmap of mean CAPE(T,H) in manuscript Figure 6, derived by taking the difference in mean CAPE and surface temperature of profiles that fall into two adjacent bins along the constant RH line. Markers denotes 'Warm' (+) and 'Hot' (x) bins used as examples in manuscript. Fractional changes for selected bins are shown in Table S5.

| | T (K) | H (g/kg) | RH (%) | CAPE (J/kg) | $\frac{dC/C}{dT}\|_{RH}$ (%/K) |
|---|---|---|---|---|---|
| 'Cool' | 286.5 | 6.1 | 64 | 22 | 11.0 |
| 'Warm' | 298.5 | 12.8 | 63 | 563 | 28.3 |
| 'Hot' | 308.5 | 16.9 | 46 | 2540 | 18.4 |
| 'Humid' | 304.5 | 20.9 | 72 | 3328 | 22.5 |

Table S5: Rate of change of SBCAPE with temperature at fixed RH in IGRA radiosondes, for selected conditions. Values shown in last column are the slope of the response surface in manuscript Figure 6, also shown in Figure S11, bottom. Middle two rows show the 'Warm' and 'Hot' bins as in manuscript Figure 7; we also show selected cases at lower temperature ('Cool') and higher humidity ('Humid'). Effective dependence of CAPE with temperature exceeds Clausius-Clapeyron in all cases.

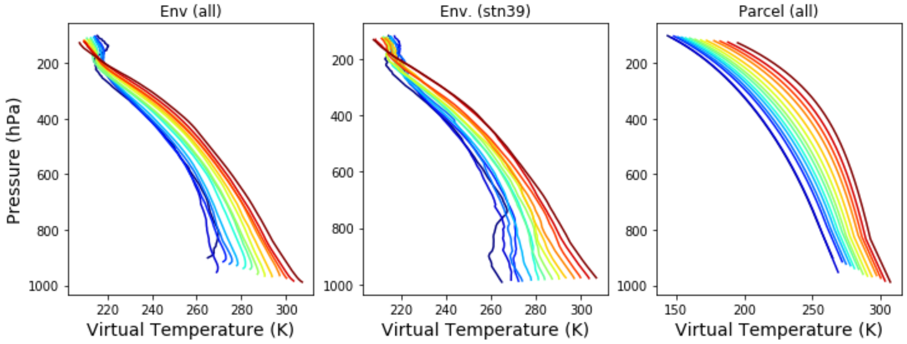


Figure S12: Demonstration of differences in temperature profiles under current climate in WRF output, for profiles with surface RH between 49–51%, binned in 3K increments. (Left) Mean environmental profiles over all stations in the dataset (MJJA 2001-2012). Note that profiles with cooler surface temperature tend to occur in higher-altitude stations with lower surface pressures. (Middle) As in left panel but for a single representative station ("TOP", Topeka, Kansas, mean CAPE 800 J/kg). (Right) Mean adiabatic profile of rising parcels initialized at 50% RH. Environmental lapse rates become steeper at warmer surface temperatures since upper tropospheric temperature are more homogeneous. This effect is comparable in magnitude to the changing lapse rate in the rising parcel, contributing to "super-Clausius-Clapeyron" CAPE scaling.
